# Supplementary material for: Resonance Fluorescence from a two-level artificial atom strongly coupled to a single-mode cavity
Source: arXiv:2202.12080 source file (2023-04-12)
Supplement: Supplementary file 1 [file Supplement_2023March27.tex]

\makeatletter
\documentclass[aps,onecolumn,prl,superscriptaddress,amsmath,showpacs,longbibliography,tightenlines]{revtex4-1}
\usepackage{graphicx}
\usepackage{bm}
\usepackage{amssymb}
\usepackage{float}
\usepackage{amsmath}

\usepackage{color}

\begin{document}

%\small

\title{Supplementary Information for "Resonance Fluorescence from a Two-level Artificial Atom Strongly Coupled to a Single-mode Cavity"}
\author{Z.H. Peng}\email{zhihui.peng@riken.jp}
\affiliation{Key Laboratory of Low-Dimensional Quantum Structures
and Quantum Control of Ministry of Education, Department of Physics
and Synergetic Innovation Center for Quantum Effects and
Applications, Hunan Normal University, Changsha 410081, China}
\affiliation{Center for Emergent Matter Science, RIKEN, Wako, Saitama 351-0198, Japan}
\author{D. He}
\affiliation{Key Laboratory of Low-Dimensional Quantum Structures
and Quantum Control of Ministry of Education, Department of Physics
and Synergetic Innovation Center for Quantum Effects and
Applications, Hunan Normal University, Changsha 410081, China}
\author{Y. Zhou}\affiliation{Center for Emergent Matter Science, RIKEN, Wako, Saitama 351-0198, Japan}
\author{J.H. Ding}
\affiliation{ School of integrated circuits,Tsinghua University,
Beijing 100084, China}
\author{J. Lu}\affiliation{Key Laboratory of Low-Dimensional Quantum Structures
and Quantum Control of Ministry of Education, Department of Physics
and Synergetic Innovation Center for Quantum Effects and
Applications, Hunan Normal University, Changsha 410081, China}
\author{L. Zhou}\affiliation{Key Laboratory of Low-Dimensional Quantum Structures
and Quantum Control of Ministry of Education, Department of Physics
and Synergetic Innovation Center for Quantum Effects and
Applications, Hunan Normal University, Changsha 410081, China}
\author{Jie-Qiao Liao}\affiliation{Key Laboratory of Low-Dimensional Quantum Structures
and Quantum Control of Ministry of Education, Department of Physics
and Synergetic Innovation Center for Quantum Effects and
Applications, Hunan Normal University, Changsha 410081, China}
\author{L.M. Kuang}\affiliation{Key Laboratory of Low-Dimensional Quantum Structures
and Quantum Control of Ministry of Education, Department of Physics
and Synergetic Innovation Center for Quantum Effects and
Applications, Hunan Normal University, Changsha 410081, China}
\affiliation{Synergetic Innovation Academy for Quantum Science and Technology, Zhengzhou University of Light Industry, Zhengzhou 450002, China}
\author{Yu-xi Liu}\email{yuxiliu@mail.tsinghua.edu.cn}
\affiliation{ School of integrated circuits,Tsinghua University,
Beijing 100084, China}
\affiliation{Beijing National Research Center for Information Science and Technology (BNRist),
Beijing 100084, China}
\author{Oleg V. Astafiev}
\email{oleg.astafiev@rhul.ac.uk}
\affiliation{Skolkovo Institute of Science and Technology, Nobel str. 3, Moscow, 143026, Russia}
\affiliation{Moscow Institute of Physics and Technology, Institutskiy Pereulok 9, Dolgoprudny 141701, Russia}
\affiliation{Royal Holloway, University of London, Egham Surrey TW20 0EX, United Kingdom}
\affiliation{National Physical Laboratory, Teddington, TW11 0LW, United Kingdom}
\author{J.S. Tsai}
\affiliation{Department of Physics, Tokyo University of Science, Kagurazaka, Tokyo 162-8601, Japan}
\affiliation{Center for Emergent Matter Science, RIKEN, Wako, Saitama 351-0198, Japan}
\maketitle

\section{The effect of Rayleigh-scattered signals in the resonance fluorescence spectrum}
The Rayleigh-scattering process results in elastic and inelastic waves (coherent and incoherent) in the resonance fluorescence \cite{Astafiev2010,Lang2011}. The resonance fluorescence (inelastic scattering) is measured with a spectrum analyzer. In the resonance fluorescence spectrum measurements, it is easier to exclude the effect of coherent signals with narrower measurement bandwidth. However, it would take longer time to get spectrum data due to lower measured signal within the narrow bandwidth. In the experiment, we set the measurement bandwidth to around a few MHz to balance the measurement time and reduce the effect of coherent signals. Furthermore, the coherent signals can be reduced by sending coherent signals with $\pi$-phase shift, but it is difficult to completely cancel them. In Fig.~\ref{RayleighEmiss}a, we present simulation of the emission spectrum including elastic and coherent signals with measurement bandwith set as $1.25\,$MHz. In Fig.~\ref{RayleighEmiss}b, we present simulation of the inelastic emission spectrum. It is shown that the central peak width in Fig.~\ref{RayleighEmiss}a is smaller than that in Fig.~\ref{RayleighEmiss}b. Therefore, we believe the slight difference between the measured linewidth of the central peak, $2\pi\times3.6\,$MHz, in Fig. 3c and $\Gamma_1/2\pi=4.8\,$MHz comes from the residual coherent signals in experiment.

There are two ways of measuring emission spectrum due to inelastic wave scattering, such as Mollow spectrum. One is to use a spectrum analyzer like it is done in our work and in Ref.~ \cite{Astafiev2010}. The advantage of this method is easy calibration of the emission spectrum density based on the noise temperature of measurement setup (supplementary in Ref.~\cite{Astafiev2010}). The disadvantage is the difficulty in excluding coherent signals because of the limited measurement bandwidth for balancing spectrum scanning speed. Another method is to use a digitizer to record signals as a function of time and then calculate the Fourier transforms of the time-dependent signals to get emission spectrum like in the work of Ref.~\cite{Lang2011}. The advantage of this method is that it is easy to exclude the coherent signals with a narrow measurement bandwidth (it is a point in Fig. 1b in Ref.~\cite{Lang2011}). However, the emission spectrum density normally can not be calibrated directly.

\begin{figure}
\center
\includegraphics[scale=1]{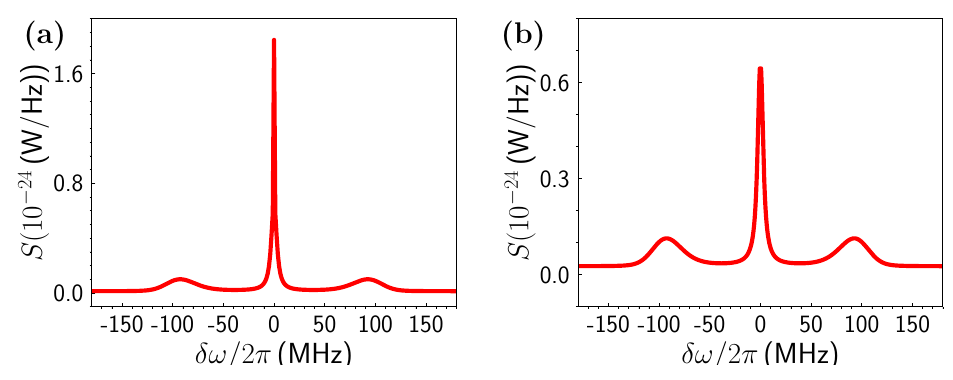}
\caption{(a) The simulated emission spectrum with elastic and coherent signals, where the measurement bandwidth is set as $1.25\,$MHz. (b) The simulated inelastic emission spectrum. }
\label{RayleighEmiss}
\end{figure}

\section{Derivation of spectrum}
%\subsection{Subsection if needed}

We consider dressed states
\begin{eqnarray}\label{rcl}
\begin{array}{rcl}
%\begin{equation}\label{rcl}
&|n,+\rangle = \frac{|n\rangle|0\rangle + |n-1\rangle|1\rangle}{\sqrt2},\\
\\
&|n,-\rangle = \frac{|n\rangle|0\rangle - |n-1\rangle|1\rangle}{\sqrt2}
%\end{equation}
\end{array}
\end{eqnarray}
describing a two-level atom coupled to a resonator in the resonance. The levels of a subsystem with four nearest states ($|n,+\rangle$, $|n,-\rangle$, $|n-1,+\rangle$ and $|n-1,-\rangle$) are shown in Fig.~\ref{Dst}.
We are also interested in the case of a large mean photon number ($\langle n\rangle \gg 1$). Four possible transitions in the system shown in the figure are possible due to relaxation of the atom described by a lowering operator $\sigma_{01} = |0\rangle\langle 1|$. The corresponding transition matrix elements are
\begin{subequations}
\begin{eqnarray}
&|n,+\rangle \rightarrow |n-1,+\rangle:\quad       \langle n-1,+|0\rangle\langle 1|n,+\rangle &= \frac{1}{2}\langle n-1,0|0\rangle\langle 1|n-1,1\rangle = \frac{1}{2} ,\\
&|n,-\rangle \rightarrow |n-1,-\rangle:\quad       \langle n-1,-|0\rangle\langle 1|n,-\rangle &= -\frac{1}{2}\langle n-1,0|0\rangle\langle 1|n-1,1\rangle = -\frac{1}{2} ,\\
&|n,+\rangle \rightarrow |n-1,-\rangle:\quad       \langle n-1,-|0\rangle\langle 1|n,+\rangle &= -\frac{1}{2}\langle n-1,0|0\rangle\langle 1|n-1,1\rangle = -\frac{1}{2}, \\
&|n,-\rangle \rightarrow |n-1,+\rangle:\quad       \langle n-1,+|0\rangle\langle 1|n,-\rangle &= \frac{1}{2}\langle n-1,0|0\rangle\langle 1|n-1,1\rangle = \frac{1}{2}.
\end{eqnarray}
\end{subequations}
All the transitions have the same value of matrix elements, which result in the factor 1/4 in the spectral density.

\begin{figure}
\center
\includegraphics[scale=1]{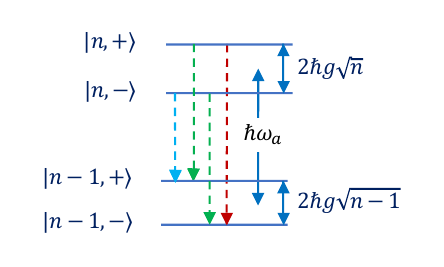}
\caption{Four possible processes of relaxation of the dressed state through the atom. }
\label{Dst}
\end{figure}

The corresponding frequencies of the transitions $|n-1,+\rangle \rightarrow |n,+\rangle$ and $|n-1,-\rangle \rightarrow |n,-\rangle$ are
$(E_{n,\pm} - E_{n-1,\pm})/\hbar = \omega_a \pm g(\sqrt n - \sqrt{n-1})$. When $g/\sqrt n \leq \Gamma_1$ (in our experiment this is fulfilled already with a very few photons), these transitions result in a central emission peak at $\omega_a$ with the width $\Gamma_1$ determined by the atom spontaneous emission to the line and the power density in maximum is
$\sim\hbar\omega_a$. Therefore the central peak with large mean photon number $\langle n\rangle$ is similar to the central peak of the standard Mollow triplet and the power spectral density can be written as
\begin{equation}
S_c(\omega) = \frac{1}{2\pi}\frac{\hbar\omega_a \Gamma_1}{4} \frac{\Gamma_1} {(\omega - \omega_a)^2 + (\Gamma_1/2)^2}.
\end{equation}
The factor $1/4$ is a result of two out of four processes contributing to the central peak (factor 1/2) and another factor 1/2 comes from the projection of the dressed states on the atomic states $|0\rangle$ and $|1\rangle$.

Two other transitions $|n,+\rangle \rightarrow |n-1,-\rangle$ and $|n,-\rangle \rightarrow |n-1,+\rangle$ (blue and red dashed lines in Fig.~4(a)) result in the appearance of sidebands with frequencies $(E_{n,+} - E_{n-1,-})/\hbar = \omega_a + g(\sqrt n + \sqrt{n-1})$ and $(E_{n,-} - E_{n-1,+})/\hbar = \omega_a - g(\sqrt n + \sqrt{n-1})$.
The processes are accompanied by changing two quantum numbers: the photon number together with the atomic state.
In that case the transition frequencies of the side peaks are shifted according to $\delta\omega_{sn} \approx g(n-\langle n\rangle)/\langle n\rangle$ in respect to the central frequency at $\omega_s$, where $\omega_s = 2g\sqrt{\langle n\rangle}$ and the Poissonian photon distribution is approximated by the Gaussian
\begin{equation}
P(n) = \frac{1}{\sqrt{2\pi \langle n\rangle}}\exp\Big[-\frac{(n - \langle n\rangle)^2}{2\langle n\rangle}\Big].
\label{Pn}
\end{equation}
Therefore, the distribution can be rewritten through frequencies according to $P(\omega_{sn})d\omega_{sn} = P(n)dn$ as
\begin{equation}
P(\omega_{sn}) = \frac{1}{\sqrt{2\pi}g}\exp\Big[-\frac{1}{2}\Big(\frac{\omega_{sn} - \omega_a\pm\omega_s}{g}\Big)^2\Big].
%P(\omega_{sn}) = \frac{1}{g\sqrt{2\pi}}\exp\Big[-\frac{1}{2}\frac{\delta\omega_{sn}^2}{g^2}\Big].
\label{Pn}
\end{equation}
The spectral density for  can be calculated as $S_s(\omega) =  (1/8)\hbar\omega_a\Gamma_1 P(\omega)$ and we arrive to
\begin{equation}
%S(\omega) = \sqrt{\frac{2}{\pi}} \frac{1}{\Delta n} \exp\Big[-\Big(\frac{2\delta n}{\Delta n}\Big)^2\Big] \times \hbar\omega\Gamma_1 2 g \sqrt{n}   ,
S_s(\omega) = \frac{1}{2\pi} \frac{\hbar\omega_a\Gamma_1}{8} \frac{\sqrt{2\pi}}{g} \exp\Big[-\frac{1}{2}\Big(\frac{\omega - \omega_a \pm \omega_s}{g}\Big)^2\Big].
\end{equation}
The factor 1/8 is a result of product of (i) the projection of the dressed states on the atomic state (1/2); (ii) one out four processes contributing to the side bands (1/4). The processes are denoted by blue and red dashed lines in Fig.~4(a).

\begin{figure}
\center
\includegraphics[scale=0.4]{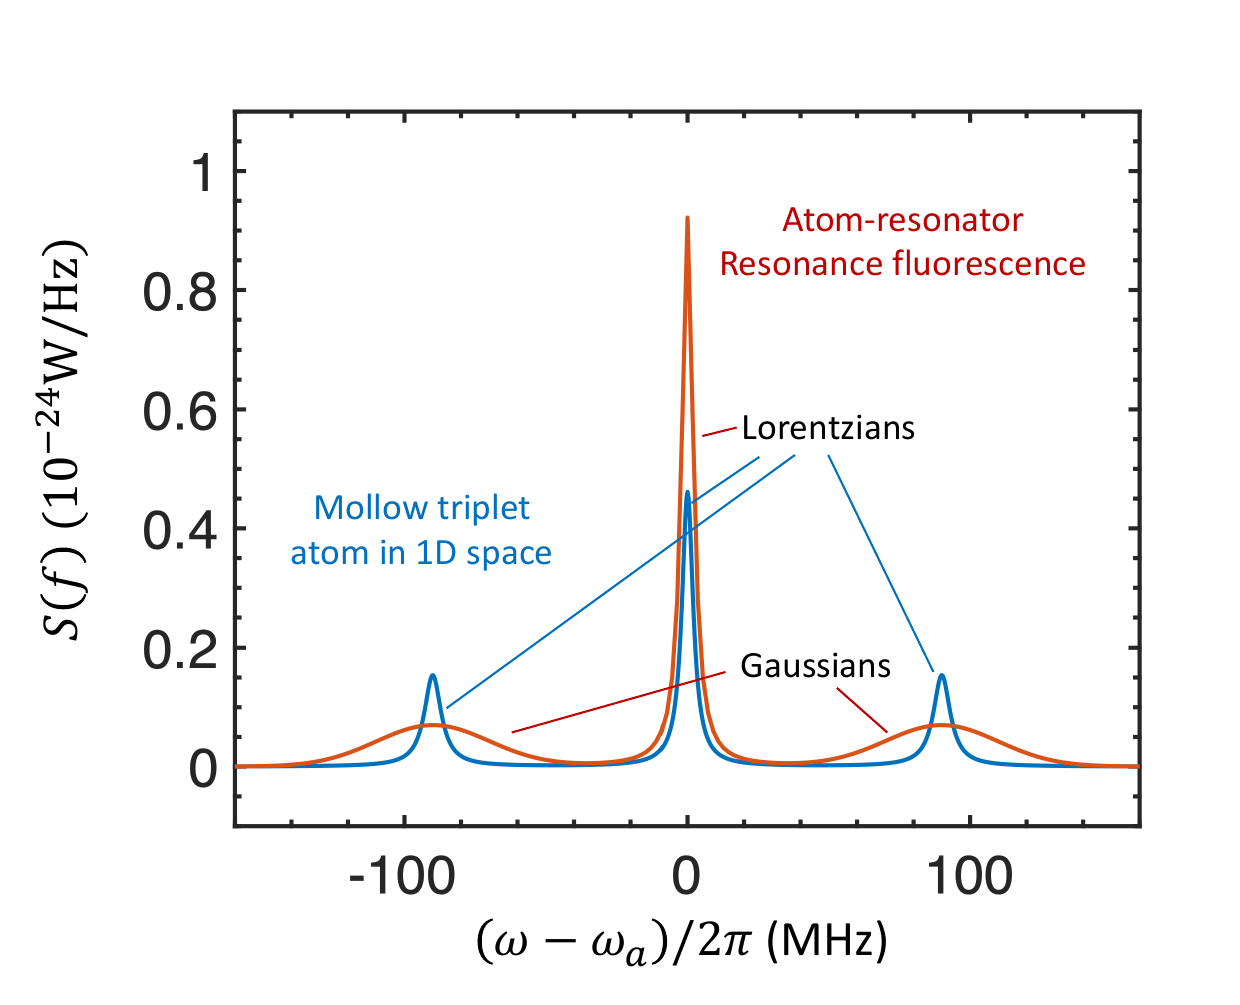}
\caption{Calculated spectra of resonance fluorescence: Blue curve: Mollow triplet from an artificial atom coupled to a transmission line with $\Gamma_1/2\pi =  4.8$~MHz. Red curve: Resonance fluorescence triplet from an atom coupled to a resonator with $g/2\pi = 20$~MHz.}
\label{S}
\end{figure}

The total spectrum is
\begin{equation}
%S(\omega) =  \frac{\hbar\omega_a\Gamma_1}{8} \Big\{ \frac{\sqrt{2\pi}}{g} \exp^{\Big[-\frac{1}{2}\Big(\frac{\omega + \omega_s}{g}\Big)^2\Big]} + \frac{2\Gamma_1}{(\omega - \omega_a)^2 + (\Gamma_1/2)^2} \frac{\sqrt{2\pi}}{g} \exp\Big[-\frac{1}{2}\Big(\frac{\omega - \omega_s}{g}\Big)^2\Big] \Big\}.
S(\omega) \approx  \frac{1}{2\pi}\frac{\hbar\omega_a\Gamma_1}{4} \Big[ \frac{\sqrt{2\pi}}{2g} e^{-\frac{1}{2}\big(\frac{\omega - \omega_a + \omega_s}{g}\big)^2} + \frac{\Gamma_1}{(\omega - \omega_a)^2 + (\Gamma_1/2)^2} + \frac{\sqrt{2\pi}}{2g} e^{-\frac{1}{2}\big(\frac{\omega  - \omega_a - \omega_s}{g}\big)^2} \Big],
\label{S0}
\end{equation}
compared with the standard Mollow triplet from an atom strongly coupled to the open 1D space~\cite{Astafiev2010},
\begin{equation}
 S(\omega) \approx  \frac{1}{2\pi} \frac{\hbar \omega_a \Gamma_1}{8} \left( \frac{\gamma_s}{(\delta \omega + \Omega)^2 +\gamma_s^2} \right.\\
     \left. +\frac{\Gamma_1}{\delta\omega^2 +(\Gamma_1/2)^2} + \frac{\gamma_s}{(\delta\omega - \Omega)^2 +\gamma_s^2} \right),
\label{S1}
\end{equation}
where $\gamma_s = 3\Gamma_1/4$ and $\Omega$ is the driving amplitude (Rabi frequency) from the classical wave.
Note that the total power in case Eq.~(\ref{S0}) ($\int S(\omega)d\omega$) is $\hbar\omega_a\Gamma_1/2$ due to half atom population and in Eq.~(\ref{S1}) is $\hbar\omega_a\Gamma_1/4$ because the scattered waves additionally leak in two directions.

%\begin{equation}
%    \nonumber S(\omega) \approx  \frac{1}{2\pi} \frac{\hbar \omega \Gamma_1}{8} \left( \frac{\gamma_s}{(\delta \omega + \Omega)^2 +\gamma_s^2} \right.\\
%     \left. +\frac{2\gamma_c}{\delta\omega^2 +\gamma_c^2} + \frac{\gamma_s}{(\delta\omega - \Omega)^2 +\gamma_s^2} \right),
%\end{equation}

\section{The sideband broaden}
In Fig.~\ref{EmissionWithDephasing}, we compare the theoretic simulation of the emission spectrum with (black square) or without (red dot) atomic dephasing effect, respectively. The atomic dephasing rate is estimated $\Gamma_{\phi}=2\pi\times1.4\,$MHz from $60\%$ quantum efficiency. We find there is around $2\,$MHz sideband peak broaden when the dephasing rate is taken into account. Also, it takes around one hour to scan and average the resonance fluorescence spectrum like in Fig.3 through the spectrum analyzer when the measurement bandwidth is set to around few MHz. The low frequency noise also could induce side peak broadening.

\begin{figure}
\center
\includegraphics[scale=1]{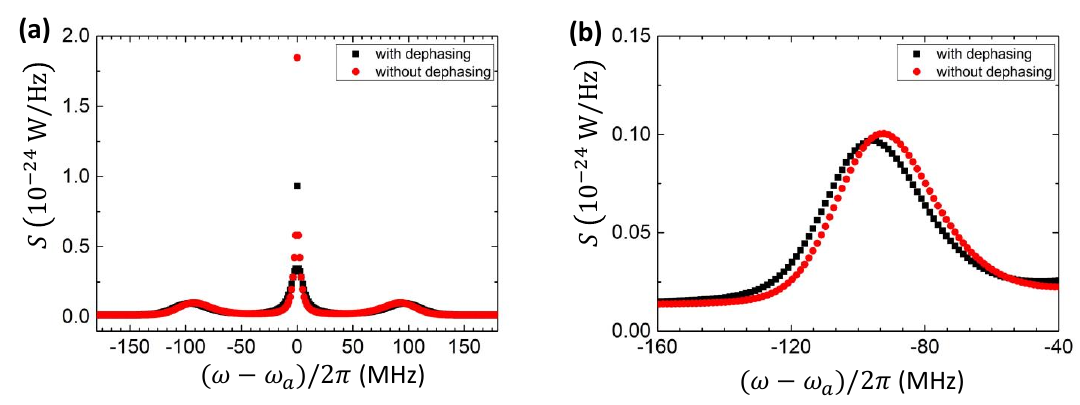}
\caption{(a) Theoretic simulation of the emission spectrum with (black square) or without dephasing effect (red dot). (b) The left sideband peaks in (a) are magnified. We can extract that the sideband peak when we take the atomic dephasing rate $\Gamma_\phi=/2\pi~1.4\,$MHz into account is $2\,$MHz wider than that without dephasing effect. }
\label{EmissionWithDephasing}
\end{figure}

\end{document}
